# Supplementary material for: Spectral rate theory for projected two-state kinetics
Source: arXiv:1207.0225 source file (2013-11-06)
Supplement: Supplementary file 1 [file SpectralRateTheory_Revision3_SI.pdf]

# Spectral rate theory for projected two-state kinetics
# Supplementary Information

Jan-Hendrik Prinz,[1] John D. Chodera,[2] and Frank Noé*[1,*]

[1]*DFG Research Center Matheon, Free University Berlin, Arnimallee 6, 14195 Berlin, Germany*[†]

[2]*Computational Biology Center, Memorial Sloan-Kettering Cancer Center, New York, NY 10065, USA*[‡]

## I. BASICS

### A. Autocorrelation of the exact eigenfunction $\psi_2$

The autocorrelation function of the exact second eigenfunction is given by:

$$\begin{aligned}\lambda_2(\tau) = \langle\psi_2(x_t)\psi_2(x_{t+\tau})\rangle_t &= \int d\mathbf{x}\int d\mathbf{y} c_\tau(\mathbf{x},\mathbf{y};\tau)\psi_2(\mathbf{x})\psi_2(\mathbf{y}) \\ &= \langle\psi_2,\mu\rangle^2 + e^{-\kappa_2\tau}\langle\psi_2,\psi_2\rangle_\mu + \sum_{i>2} e^{-\kappa_i\tau}\langle\psi_2,\psi_i\rangle_\mu \\ &= e^{-\kappa_2\tau}, \end{aligned} \tag{1}$$

using orthogonality of the eigenfunctions $\psi_i$ results in:

$$\begin{aligned}\lambda_2(\tau) &= \langle\psi_2,\mu\rangle^2 + e^{-\kappa_2\tau}\langle\psi_2,\psi_2\rangle_\mu + \sum_{i>2} e^{-\kappa_i\tau}\langle\psi_2,\psi_i\rangle_\mu \\ &= e^{-\kappa_2\tau}, \end{aligned} \tag{2}$$

such that the single-$\tau$ rate estimate

$$\hat{\kappa}_2 = -\frac{\ln\lambda_2(\tau)}{\tau} = \kappa_2 \tag{3}$$

is exact (without a systematic error).

### B. Autocorrelation of model functions $\tilde{\psi}_2$

We take an arbitrary function $\tilde{\psi}_2$. Throughout this paper, $\tilde{\psi}_2$ is subject to the normalization conditions

$$\begin{aligned}\langle\tilde{\psi}_2,\mu\rangle &= 0 \\ \langle\tilde{\psi}_2,\tilde{\psi}_2\rangle &= 1, \end{aligned} \tag{4}$$

that shall serve as a model for $\psi_2$. Using the shorthand notation

$$a_i = \langle\tilde{\psi}_2,\psi_i\rangle \tag{5}$$

we expand $\tilde{\psi}_2$ in terms of eigenfunctions $\psi_i$:

$$\begin{aligned}\tilde{\psi}_2 &= \sum_i a_i\psi_i \\ &= a_2\psi_2 + \sum_{i>2} a_i\psi_i \\ &= \sqrt{\alpha}\psi_2 + \sum_{i>2} a_i\psi_i \end{aligned} \tag{6}$$

---

*Electronic address: frank.noe@fu-berlin.de

†Electronic address: jan-hendrik.prinz@fu-berlin.de

‡Electronic address: choderaj@mskcc.org

Parseval's identity gives:

$$\sum_i a_i^2 = 1. \tag{7}$$

And thus:

$$\begin{aligned}
\tilde{\lambda}_2(\tau) = \langle \tilde{\psi}_2(0)\tilde{\psi}_2(\tau)\rangle &= a_2^2\lambda_2(\tau) + \sum_{i>2} a_i^2\lambda_i(\tau) \\
&= a_2^2\lambda_2(\tau) + \lambda_3(\tau)\sum_{i>2} a_i^2 \frac{\lambda_i(\tau)}{\lambda_3(\tau)} \\
&\leq a_2^2\lambda_2(\tau) + (1-a_2^2)\lambda_3(\tau) \\
&= \alpha\lambda_2(\tau) + (1-\alpha)\lambda_3(\tau)
\end{aligned} \tag{8}$$

### C. Observed dynamics

Let $\chi(y \mid \mathbf{x})$ be the output probability density, providing the conditional density of observing a point $y \in \mathbb{R}$ given that the full-space configuration of the system is $\mathbf{x} \in \Omega$. Using $\phi_i(\mathbf{x}) = \mu(\mathbf{x})\psi_i(\mathbf{x})$ as the $i$-th eigenfunction scaled by the stationary density, we can express the correlation density of observing the system at point $y_0$ at time 0 and at time $y_\tau$ a time $\tau$ later as:

$$\begin{aligned}
c_\tau(y_0, y_\tau) &= \int d\mathbf{x}_0 \int d\mathbf{x}_\tau\, \chi(y_0 \mid \mathbf{x}_0) c_\tau(\mathbf{x}_0, \mathbf{x}_\tau)\chi(y_\tau \mid \mathbf{x}_\tau) \\
&= \sum_{i=1}^{\infty} \lambda_i(\tau) \int d\mathbf{x}_0\, \chi(y_0 \mid \mathbf{x}_0)\phi_i(\mathbf{x}_0) \int d\mathbf{x}_\tau\, \phi_i(\mathbf{x}_\tau)\chi(y_\tau \mid \mathbf{x}_\tau) \\
&= \sum_{i=1}^{\infty} \lambda_i(\tau)\phi_i^y(y_0)\phi_i^y(y_\tau) \\
&= \mu^y(y_0)\mu^y(y_\tau) + \sum_{i=2}^{\infty} \lambda_i(\tau)\phi_i^y(y_0)\phi_i^y(y_\tau)
\end{aligned} \tag{9}$$

Here, we have defined the observed (projected) eigenfunctions

$$\phi_i^y(y) = \int d\mathbf{x}\, \chi(y \mid \mathbf{x})\phi_i(\mathbf{x}) \tag{10}$$

$$\psi_i^y(y) = \int d\mathbf{x}\, \chi(\mathbf{x} \mid y)\psi_i(\mathbf{x}) \tag{11}$$

using

$$\chi(\mathbf{x} \mid y)\mu^y(y) = \chi(y \mid \mathbf{x})\mu(\mathbf{x}) \tag{12}$$

and the special case for the stationary distribution:

$$\mu^y(y) = \phi_1^y(y) = \int d\mathbf{x}\, \chi(y \mid \mathbf{x})\mu(\mathbf{x}). \tag{13}$$

All observed eigenfunctions with $i > 1$ are still orthogonal to the observed stationary distribution with respect to the observed stationary distribution $\mu^y(y)$:

$$\begin{aligned}
\langle \psi_i^y(y), \mu^y(y)\rangle &= \int dy\, \mu^y(y) \int d\mathbf{x}\, \chi(\mathbf{x} \mid y)\psi_i(\mathbf{x}) \\
&= \int dy \int d\mathbf{x}\, \chi(y \mid \mathbf{x})\mu(\mathbf{x})\psi_i(\mathbf{x}) \\
&= \int d\mathbf{x}\, \mu(\mathbf{x})\psi_i(\mathbf{x}) \\
&= 0
\end{aligned} \tag{14}$$

where we assume that the output probabilities are complete

$$\int dy\, \chi(y \mid \mathbf{x}) = 1, \tag{15}$$

i.e., for each state $\mathbf{x}$ the total probability to observe any $y$ is one. Similarly we derive that

$$\int d\mathbf{x}\, \chi(\mathbf{x} \mid y) = \int d\mathbf{x}\, \frac{\chi(y \mid \mathbf{x})\mu(\mathbf{x})}{\mu^y(y)} = \frac{\mu^y(y)}{\mu^y(y)} = 1 \tag{16}$$

holds. Let us now concentrate on the two-state case, i.e., we assume that a time-scale separation exists between $t_2 = \kappa_2^{-1}$ and $t_3 = \kappa_3^{-1}$, such that at the lag times of interest all eigenvalues $\lambda_i(\tau) \approx 0$ with $i > 2$. Thus, we can express the propagator in terms of only two dominant eigenfunctions, $\mu$ and $\phi_2$, and their projected counterparts, $\mu^y$ and $\phi_2^y$. The norm of the observed eigenfunction $\phi_2^y$ with respect to the projected stationary distribution is:

$$\begin{aligned}
\hat{\alpha}_y = \langle \phi_2^y, \psi_2^y \rangle &= \int dy \int d\mathbf{x}_1\, \chi(y \mid \mathbf{x}_1)\phi_2(\mathbf{x}_1) \int d\mathbf{x}_2\, \chi(\mathbf{x}_2 \mid y)\psi_2(\mathbf{x}_2) \\
&= \int d\mathbf{x}_1 \int d\mathbf{x}_2\, \phi_2(\mathbf{x}_1) \left( \int dy\, \chi(\mathbf{x}_2 \mid y)\chi(y \mid \mathbf{x}_1) \right) \psi_2(\mathbf{x}_2) \\
&= \int d\mathbf{x}_1 \int d\mathbf{x}_2\, \phi_2(\mathbf{x}_1)\mathcal{M}(\mathbf{x}_1,\mathbf{x}_2)\psi_2(\mathbf{x}_2) \\
&\equiv \langle \phi_2^y, \psi_2^y \rangle_{\mathcal{M}}
\end{aligned} \tag{17}$$

where $\mathcal{M}$ is a mixing kernel that contains the induced overlap in the original space due to the output probabilities $\chi$.

### D. Reaction coordinate quality and observation quality

Now we consider approximating the second eigenvalue of the two-state system by a probe function $\tilde{\psi}_2$:

$$\begin{aligned}
\langle \tilde{\psi}_2(y_t)\tilde{\psi}_2(y_{t+\tau}) \rangle_t &= \langle \tilde{\psi}_2, \mu^y \rangle^2 + \lambda_2(\tau)\langle \tilde{\psi}_2, \phi_2^y \rangle^2 \\
&= \lambda_2(\tau)\langle \tilde{\psi}_2, \phi_2^y \rangle^2 \\
&= \alpha\lambda_2(\tau)
\end{aligned} \tag{18}$$

with $\alpha = \langle \tilde{\psi}_2, \phi_2^y \rangle^2$. In the spectral estimation method, we choose the probe function $\tilde{\psi}_2$ to be the second eigenfunction $\hat{\psi}_2$ of an observable transition kernel

$$p_\tau(y_1, y_2) = \mu^y(y_1)^{-1} c_\tau(y_1, y_2). \tag{19}$$

This second eigenvector $\hat{\psi}_2$ is normalized and orthogonal to the observed stationary distribution

$$\langle \hat{\psi}_2(y), \mu^y(y) \rangle = 0 \tag{20}$$

$$\langle \hat{\psi}_2(y), \hat{\psi}_2(y) \rangle_{\mu^y} = 1, \tag{21}$$

maximizes the estimated second eigenvalue $\hat{\lambda}_2(\tau)$ under the given orthogonality constraints and with RCQ

$$\hat{\alpha}_y = \langle \hat{\psi}_2, \phi_2^y \rangle = \langle \phi_2^y, \psi_2^y \rangle. \tag{22}$$

Now we ask about the magnitude of $\hat{\alpha}_y$ depending on the type of the observation $\chi$, or the mixing matrix $\mathcal{M}$. For perfect RC's, every $y$ is uniquely associated with one $\mathbf{x}$, i.e., $\chi$ is a bijective map and

$$\mathcal{M}(\mathbf{x}_1, \mathbf{x}_2) = \delta(\mathbf{x}_1, \mathbf{x}_2) \tag{23}$$

in this case we get:

$$\hat{\alpha}_{\text{y,perfect}} = \int d\mathbf{x}_1 \int d\mathbf{x}_2\, \phi_2(\mathbf{x}_1)\delta(\mathbf{x}_1, \mathbf{x}_2)\psi_2(\mathbf{x}_2) = \langle \psi_2, \phi_2 \rangle = 1. \tag{24}$$

For all other cases we view $\mathcal{M}$ as a transition operator that reduces $\hat{\alpha}_y$ by projecting eigenfunctions, such that the projected eigenfunction has a reduced norm. Consider the following properties of $\mathcal{M}$:

1. $\mathcal{M}$ is a transition operator. Proof:
$$\int d\mathbf{x}_2\,\mathcal{M}(\mathbf{x}_1,\mathbf{x}_2) \;=\; \int d\mathbf{x}_2\int dy\,\chi(\mathbf{x}_2\mid y)\chi(y\mid\mathbf{x}_1)=\int dy\,\chi(y\mid\mathbf{x}_1)=1. \tag{25}$$

2. $\mathcal{M}$ fulfills detailed balance with respect to $\mu$. Proof:
$$\begin{aligned}\mu(\mathbf{x}_1)\mathcal{M}(\mathbf{x}_1,\mathbf{x}_2) &= \mu(\mathbf{x}_1)\int dy\,\chi(\mathbf{x}_2\mid y)\chi(y\mid\mathbf{x}_1)\\ &= \int dy\,\chi(\mathbf{x}_2\mid y)\mu^y(y)\chi(\mathbf{x}_1\mid y)\\ &= \mu(\mathbf{x}_2)\int dy\,\chi(\mathbf{x}_1\mid y)\chi(y\mid\mathbf{x}_2)\\ &= \mu(\mathbf{x}_2)\mathcal{M}(\mathbf{x}_2,\mathbf{x}_1)\end{aligned} \tag{26}$$

3. $\mu(\mathbf{x})$ is a stationary density of $\mathcal{M}$. Proof:
$$\int d\mathbf{x}_1\,\mu(\mathbf{x}_1)\mathcal{M}(\mathbf{x}_1,\mathbf{x}_2) \;=\; \mu(\mathbf{x}_2)\int d\mathbf{x}_1\,\mathcal{M}(\mathbf{x}_2,\mathbf{x}_1)=\mu(\mathbf{x}_2)$$

4. As a result, we can decompose $\mathcal{M}$ into its spectral components:
$$\mathcal{M}=\sum_{i=1}^{\infty}\beta_i\frac{l_i(\mathbf{x}_1)}{\mu(\mathbf{x}_1)}l_i(\mathbf{x}_2) \tag{27}$$
with $\beta_i\le 1$ being the eigenvalues and $l_i$ being the eigenfunctions. Note that $\mathcal{M}$ is not necessarily irreducible and may thus have multiple 1-eigenvalues. For example, a projective $\mathcal{M}$ will have multiple 1-eigenvalues as it does not mix between different values of $y$. A dispersive $\mathcal{M}$ will typically be irreducible and thus have a unique eigenvalue $\beta_1=1$.

From these properties and the fact that transition operators have a spectral radius of one, it directly follows that
$$\begin{aligned}\hat{\alpha}_y &= \langle\phi_2,\psi_2\rangle_{\mathcal{M}}\\ &= \int d\mathbf{x}_1\psi_2(\mathbf{x}_1)\int d\mathbf{x}_2\sum_{i=1}^{\infty}\beta_i l_i(\mathbf{x}_1)l_i(\mathbf{x}_2)\psi_2(\mathbf{x}_2)\\ &= \le\sum_{i=2}^{\infty}\beta_i\langle\psi_2(\mathbf{x}),l_i(\mathbf{x})\rangle^2\le\beta_2\le 1\end{aligned}$$
where from property (2) follows that $l_1(\mathbf{x})=\mu_x(\mathbf{x})$ so that $\langle l_1(\mathbf{x}),\psi_2(\mathbf{x})\rangle=0$ and the first term in the sum vanishes. Thus, the magnitude of the second eigenfunction is at best preserved when applying projection and/or dispersion, but in general decreases.

**Multiple application of projection/dispersion**

To understand the effect of two subsequent observation processes, we consider the example of applying first a projection from full configuration $\mathbf{x}$ to order parameter $y$, $\chi_p=\chi(y\mid\mathbf{x})$, and subsequently a dispersion to reach observable $o$, $\chi_d=\chi(o\mid y)$. For a two-state system, the observed correlation density in $o$ is:
$$\begin{aligned}c_\tau^o(o_0,o_\tau) &= \int dy_0\int dy_\tau\,\chi(o_0\mid y_0)\int d\mathbf{x}_0\int d\mathbf{x}_\tau\,\chi(y_0\mid\mathbf{x}_0)c_\tau(\mathbf{x}_0,\mathbf{x}_\tau)\chi(y_\tau\mid\mathbf{x}_\tau)\chi(o_\tau\mid y_\tau)\\ &= \sum_{i=1}^{\infty}\lambda_i(\tau)\int dy_0\,\chi(o_0\mid y_0)\phi_i^y(y_0)\int dy_\tau\,\chi(o_\tau\mid y_\tau)\phi_i^y(y_\tau)\\ &= \sum_{i=1}^{\infty}\lambda_i(\tau)\phi_i^o(y_0)\phi_i^o(y_\tau)\end{aligned} \tag{28}$$
where the twice-projected eigenfunctions are
$$\phi_i^o(o) \;=\; \int dy\,\chi(o\mid y)\phi_i^y(y) \tag{29}$$
$$\mu^o(o) \;=\; \int dy\,\chi(o\mid y)\mu^y(y) \tag{30}$$
$$\psi_i^o(o) \;=\; \int dy\,\chi(y\mid o)\psi_i^y(y). \tag{31}$$

For two-state systems this simplifies to

$$c^o_\tau(o_0, o_\tau) = \mu^o(o_0)\mu^o(o_\tau) + \lambda_2(\tau)\phi^o_2(y_0)\phi^o_2(y_\tau). \tag{32}$$

It follows that the observation quality (OQ) from projection and dispersion is:

$$\begin{aligned}\hat{\alpha}_o &= \langle \phi^o_2, \psi^o_2 \rangle \\ &= \langle \phi^y_2, \psi^y_2 \rangle_{\mathcal{M}_d}\end{aligned} \tag{33}$$

using the variational principle from above we can directly conclude that

$$\hat{\alpha}_o = \langle \phi^y_2, \psi^y_2 \rangle_{\mathcal{M}_d} \;\leq\; \langle \phi^y_2, \psi^y_2 \rangle = \hat{\alpha}_y. \tag{34}$$

When applying multiple subsequent projections or dispersions, the reaction coordinate quality can never increase. It at best stays the same but generally deteriorates. It does so until it reaches zero which is the OQ of white noise.

## II. CHOICES FOR MODEL FUNCTIONS $\tilde{\psi}_2$

### A. Dividing surfaces

Most rate theories operate by defining a single dividing surface which splits the state space into reactants $A$ and products $B$. Calling $h_A(y)$ the indicator function which is 1 for set $A$ and 0 for set $B$, one may define the normalized fluctuation autocorrelation function of state $A$ [5].

$$C(t) = \frac{\langle \delta h_A(0)\delta h_A(\tau)\rangle}{\langle \delta h_A^2 \rangle} \tag{35}$$

where $\delta h_A \equiv h_A - \langle h_A \rangle$. Eq. (35) can also be interpreted as the autocorrelation function

$$C(t) \;=\; \langle \tilde{\psi}_2(0)\tilde{\psi}_2(\tau)\rangle = \sum_{i=2}^{\infty} e^{-\kappa_i t} a_i^2 \tag{36}$$

for the special choice of $\tilde{\psi}_2$

$$\tilde{\psi}_{2,\mathrm{divide}}(y) = \frac{\delta h_A(y)}{\langle \delta h_A^2 \rangle^{1/2}} = \frac{h_A(y) - \pi_A}{\sqrt{\pi_A \pi_B}} = \frac{h_A(y) - \pi_A}{\sqrt{\pi_A - \pi_A^2}} \tag{37}$$

where $\pi_A = \langle h_A \rangle_\mu$ is the stationary probability of state A and $\pi_B = 1 - \pi_A$ the stationary probability of state B. To see that Eq. (37) is properly normalized, let us recall the normalization conditions:

$$\begin{aligned}\langle \tilde{\psi}_2, \mu \rangle = \langle \tilde{\psi}_2(y) \rangle &= 0 \\ \langle \tilde{\psi}_2, \tilde{\psi}_2 \rangle_\mu = \langle \tilde{\psi}_2(y)^2 \rangle &= 1\end{aligned} \tag{38}$$

For the choice (37) we get:

$$\begin{aligned}\langle \tilde{\psi}_2, \mu \rangle &= \frac{\langle h_A(y) - \pi_A \rangle_\mu}{\sqrt{\pi_A - \pi_A^2}} \\ &= \frac{\pi_A - \pi_A}{\sqrt{\pi_A - \pi_A^2}} = 0\end{aligned} \tag{39}$$

and

$$\begin{aligned}\langle \tilde{\psi}_2, \tilde{\psi}_2 \rangle_\mu &= \frac{1}{\pi_A - \pi_A^2} \langle (h_A(y) - \pi_A)(h_A(y) - \pi_A) \rangle \\ &= \frac{1}{\pi_A - \pi_A^2} \langle h_A(y)h_A(y) - \pi_A h_A(y) - \pi_A h_A(y) + \pi_A^2 \rangle_\mu \\ &= \frac{1}{\pi_A - \pi_A^2} (\pi_A - \pi_A^2 - \pi_A^2 + \pi_A^2) = 1.\end{aligned} \tag{40}$$

For the step function, we obtain the RCQ

$$\begin{aligned}
\alpha &= \langle\hat{\psi}_2, \psi_2\rangle_\mu^2 \\
&= \left\langle \frac{h_A(x) - \pi_A}{\sqrt{\pi_A - \pi_A^2}}, \psi_2 \right\rangle_\mu^2 \\
&= \frac{\left(\langle h_A(x), \psi_2\rangle_\mu - \pi_A\langle 1, \psi_2\rangle_\mu\right)^2}{\pi_A - \pi_A^2} \\
&= \frac{\langle h_A(x), \psi_2\rangle_\mu^2}{\pi_A - \pi_A^2}.
\end{aligned} \tag{41}$$

*Single-$\tau$ rate estimate.* The procedure of splitting the observed state space into two sets and estimating the transition rate from the second eigenvalue of the two-state transition matrix [2] results in a single-$\tau$ estimate (see below) with an error of

$$\hat{\kappa}_{2,\text{divide}} - \kappa_2 \leq -\frac{1}{\tau} \ln \frac{\langle h_A(x), \psi_2\rangle_\mu^2}{\pi_A - \pi_A^2} \tag{42}$$

This estimator is effectively a two-state Markov model estimate and has been analyzed in [2]. The best possible dividing surface can be chosen by maximizing $\alpha$, or equivalently, by minimizing $\tilde{\kappa}_2$. However, it is suboptimal compared to the MSM estimator that uses a finer partition of state space and thus $\tilde{\kappa}_2 \geq \hat{\kappa}_2 \geq \kappa_2$, with an error that also decays with $\tau^{-1}$.

### B. Autocorrelation of the observable

*Signal autocorrelation estimate*: Another common choice is to calculate the normalized autocorrelation function of the signal $y(t)$ itself:

$$\langle\tilde{\psi}_2(0)\tilde{\psi}_2(\tau)\rangle = \frac{\langle y(t)y(t+\tau)\rangle - \langle y\rangle^2}{\langle y^2\rangle - \langle y\rangle^2} \tag{43}$$

where we have defined $\tilde{\psi}_{2,\text{signal}}(y) = \frac{y - \langle y\rangle}{\sqrt{\langle y^2\rangle - \langle y\rangle^2}}$. To see that this function is properly normalized, consider:

$$\begin{aligned}
\langle\tilde{\psi}_2, \mu\rangle &= \frac{1}{\sqrt{\langle y^2\rangle - \langle y\rangle^2}} \int dy'\, \mu(y')y' - \mu(y')\langle y\rangle \\
&= \frac{1}{\sqrt{\langle x^2\rangle - \langle x\rangle^2}} \langle y\rangle(1 - \int dy' \mu(y')) \\
&= 0
\end{aligned} \tag{44}$$

and

$$\begin{aligned}
\langle\tilde{\psi}_2, \tilde{\psi}_2\rangle_\mu &= \int dy'\, \mu(y') \frac{(y' - \langle y\rangle))^2}{\langle y^2\rangle - \langle y\rangle^2} \\
&= \frac{1}{\langle y^2\rangle - \langle y\rangle^2} \int dy\, \mu(y')y'^2 - \mu(y')2y'\langle y\rangle + \mu(y')\langle y\rangle^2 \\
&= \frac{1}{\langle y^2\rangle - \langle y\rangle^2}(\langle y^2\rangle - 2\langle y\rangle^2 + \langle y\rangle^2) \\
&= \frac{1}{\langle y^2\rangle - \langle y\rangle^2}(\langle y^2\rangle - \langle y\rangle^2) \\
&= 1
\end{aligned} \tag{45}$$

Like for the dividing surface estimate, direct evaluation of the autocorrelation function of $\tilde{\psi}_2$ leads to a single-$\tau$ estimate of $\kappa_2$ that converges with $\tau^{-1}$ but is suboptimal compared to the MSM estimate:

$$\hat{\kappa}_{2,\mathrm{signal}} \approx \kappa_2 - \frac{1}{\tau} \ln \frac{\langle y, \psi_2 \rangle_\mu - 1}{\sqrt{\langle y^2 \rangle - \langle y \rangle^2}} \tag{46}$$

with an RCQ $\alpha < \hat{\alpha}$

$$\begin{aligned} \alpha &= \langle \hat{\psi}_2, \psi_2 \rangle_\mu^2 \\ &= \langle \frac{y - \langle y \rangle}{\sqrt{\langle y^2 \rangle - \langle y \rangle^2}}, \psi_2 \rangle_\mu^2 \\ &= \frac{1}{\langle y^2 \rangle - \langle y \rangle^2} \left( \langle y, \psi_2 \rangle_\mu - \langle y \rangle \langle 1, \psi_2 \rangle_\mu \right)^2 \\ &= \frac{\langle y, \psi_2 \rangle_\mu^2}{\langle y^2 \rangle - \langle y \rangle^2} = \frac{\langle y, \psi_2 \rangle_\mu^2}{\mathrm{Var}(y)} \end{aligned} \tag{47}$$

## III. RATE ESTIMATION METHODS

### A. Integrating the correlation function

A means of estimating the rate is to integrate the correlation function $\tilde{\lambda}_2(\tau)$ (see, e.g., Equation 3.6 of [1]),

$$\begin{aligned} \tilde{\kappa}_{2,\mathrm{int}} &= -\left( \int_0^\infty d\tau \, \tilde{\lambda}_2(\tau) \right)^{-1} \\ &= -\left( \int_0^\infty d\tau \left[ \alpha \mathrm{e}^{-\kappa_2 \tau} + \sum_{i>2} a_i^2 \mathrm{e}^{-\kappa_i \tau} \right] \right)^{-1} \\ &= -\left( \left[ \alpha \frac{1}{\kappa_2} \mathrm{e}^{-\kappa_2 \tau} + \sum_{i>2} \frac{a_i^2}{\kappa_i} \mathrm{e}^{-\kappa_i \tau} \right]_0^\infty \right)^{-1} \\ &= \left( \alpha \frac{1}{\kappa_2} + \sum_{i>2} \frac{a_i^2}{\kappa_i} \right)^{-1} \end{aligned} \tag{48}$$

with the projection amplitudes $a_i = \langle \tilde{\psi}_i, \psi_i \rangle$ and $\alpha = \langle \tilde{\psi}_2, \psi_2 \rangle_\mu^2 = a_2^2$. The reactive flux rate involves the systematic error

$$\begin{aligned} \tilde{\kappa}_{2,\mathrm{int}} - \kappa_2 &= \frac{1}{\alpha \frac{1}{\kappa_2} + \sum_{i>2} \frac{a_i^2}{\kappa_i}} - \kappa_2 \\ &= \frac{\kappa_2}{\alpha + \sum_{i>2} a_i^2 \frac{\kappa_2}{\kappa_i}} - \kappa_2 \\ &= \kappa_2 \left( \frac{1 - \alpha + \sum_{i>2} a_i^2 \frac{\kappa_2}{\kappa_i}}{\alpha + \sum_{i>2} a_i^2 \frac{\kappa_2}{\kappa_i}} \right) \\ &< \kappa_2 \left( \frac{1 - \alpha + \sum_{i>2} a_i^2}{\alpha + \sum_{i>2} a_i^2 \frac{\kappa_2}{\kappa_i}} \right) \\ &< \frac{\kappa_2 (1 - \alpha)}{\alpha + \sum_{i>2} a_i^2 \frac{\kappa_2}{\kappa_i}} \end{aligned} \tag{49}$$

where we have used Parseval's identity $\sum_{i=2}^\infty a_i^2 = 1$. For the beneficial case of a time scale separation $\kappa_2 \ll \kappa_3$, this simplifies to:

$$\Delta \kappa_{2,\mathrm{int}} = \tilde{\kappa}_{2,\mathrm{int}} - \kappa_2 \approx \kappa_2 \frac{(1 - \alpha)}{\alpha} \tag{50}$$

which becomes 0 for $\alpha = 1$, but may be very large for imperfect reaction coordinates with $\alpha < 1$.

### B. Reactive flux rate

Chandler, Montgomery and Berne [1, 4] considered the reactive flux correlation function,

$$k(\tau) \equiv -\frac{d}{dt}C(t) = \sum_{i=1}^{\infty}\langle\tilde{\psi}_2,\psi_i\rangle_\mu^2\kappa_i e^{-\kappa_i\tau} \tag{51}$$

where, for $\tau_{\text{mol}} < \tau \ll \kappa_2^{-1}$, the reactive flux $k(\tau) \approx ke^{-\kappa\tau}$, such that for $\tau \sim \tau_{\text{mol}}$ (the molecular relaxation timescale within a conformational state), the rate estimate is

$$\tilde{\kappa}_{2,\text{rf}} = \kappa_2\alpha + \sum_{i>2}\langle\tilde{\psi}_2,\psi_i\rangle_\mu^2\kappa_i e^{-\kappa_i\tau} \tag{52}$$

such that the error is given by

$$\Delta\kappa_{2,\text{rf}} = \tilde{\kappa}_{2,\text{rf}} - \kappa_2 = \kappa_2(\alpha-1) + \sum_{i>2}\langle\tilde{\psi}_2,\psi_i\rangle_\mu^2\kappa_2 e^{-\kappa_i\tau} > 0 \tag{53}$$

### C. Transition state theory

The transition state theory rate, which measures the instantaneous flux across the dividing surface between $A$ and $B$, can be computed from the short-time limit of the reactive flux [1],

$$\tilde{\kappa}_{2,\text{tst}} = k_{\text{tst}} = \lim_{t\to 0^+} k(t) = \alpha\kappa_2 + \sum_{i>2}\langle\tilde{\psi}_2,\psi_i\rangle_\mu^2\kappa_i \tag{54}$$

such that the error in the is given by

$$\Delta\kappa_2 = \tilde{\kappa}_{2,\text{tst}} - \kappa_2 = \sum_{i>2}^{\infty}\langle\tilde{\psi}_2,\psi_i\rangle_\mu^2\left(\frac{\kappa_i}{\kappa_2}-1\right) \geq \tilde{\kappa}_{2,\text{rf}} - \kappa_2 > 0 \tag{55}$$

which is either equal to or (usually) an overestimate of the true rate.

### D. Single-$\tau$ rate estimator and its systematic error

A rate estimate based on a single-$\tau$-fit of $\tilde{\lambda}_2(\tau)$ is defined as follows:

$$\begin{aligned}
\hat{\kappa}_2 &= -\tau^{-1}\ln\tilde{\lambda}_2(\tau) \\
&= -\tau^{-1}\ln\left(\alpha\lambda_2(\tau) + \sum_{i>2}a_i^2\lambda_i(\tau)\right) \\
&= -\tau^{-1}\ln\left(\alpha \mathrm{e}^{-\tau\kappa_2} + \sum_{i>2}a_i^2\mathrm{e}^{-\tau\kappa_i}\right) \\
&= -\tau^{-1}\ln\left(\mathrm{e}^{-\tau\kappa_2}\left[\alpha + \sum_{i>2}a_i^2\mathrm{e}^{-\tau(\kappa_i-\kappa_2)}\right]\right) \\
&= -\tau^{-1}\left(\ln\mathrm{e}^{-\tau\kappa_2} + \ln\left[\alpha + \sum_{i>2}a_i^2\mathrm{e}^{-\tau(\kappa_i-\kappa_2)}\right]\right)
\end{aligned} \tag{56}$$

which leads to the systematic error in the rate $\hat{\kappa}_2$:

$$\Delta\kappa_{2,\tau} = \tilde{\kappa}_{2,\tau} - \kappa_2 = -\tau^{-1}\ln\left[\alpha + \sum_{i>2}a_i^2\mathrm{e}^{-\tau(\kappa_i-\kappa_2)}\right] \tag{57}$$

Please note that the expression in the logarithm is smaller than unity, such that the rate $\hat{\kappa}_2$ is always overestimated. We can continue to simplify to

$$
\begin{aligned}
\Delta\kappa_{2,\tau} &= -\tau^{-1}\ln\left(\alpha(1+\sum_{i>2}\frac{a_i^2}{\alpha}\mathrm{e}^{-\tau(\kappa_i-\kappa_2)})\right) \\
&= \tau^{-1}\ln\frac{1}{\alpha}-\tau^{-1}\ln\left(1+\sum_{i>2}\frac{a_i^2}{\alpha}\mathrm{e}^{-\tau(\kappa_i-\kappa_2)}\right)
\end{aligned} \tag{58}
$$

as an expression for the estimation error. This error can then be bounded using $0 \leq \ln(1+x)$ for $x \geq 0$ by

$$
0 \ \leq \Delta\kappa_{2,\tau} \leq \ \tau^{-1}\ln\frac{1}{\alpha} \tag{59}
$$

and since $\kappa_i > \kappa_2$ is true for $i > 2$ we can also find a lower bound on the error that only depends on the spectral gap $\kappa_3 - \kappa_2$ and the RCQ $\alpha$

$$
0 \leq \tau^{-1}\ln\frac{1}{\alpha} - \tau^{-1}\ln\left(1+\frac{1-\alpha}{\alpha}\mathrm{e}^{-\tau(\kappa_3-\kappa_2)}\right) \ \leq \Delta\kappa_{2,\tau} \leq \ \tau^{-1}\ln\frac{1}{\alpha} \tag{60}
$$

where we used that $\ln(1+x) < x$ always holds. We conclude that the estimation error $\Delta\kappa_2$ is dominated by a $1/\tau$ dependence whereas the width of this error bound decreases exponentially in the spectral gap. For a two-state system with with a large gap $\kappa_2 \gg \kappa_3$ this uncertainty vanishes and the rate error is indeed approximated by:

$$
\Delta\kappa_{2,\tau} \approx \tau^{-1}\ln\frac{1}{\alpha}. \tag{61}
$$

### E. Multi-$\tau$ exponential fitting estimators

Exponential-fitting estimators usually employ an exponential fit to autocorrelation functions $\tilde{\lambda}_2(\tau)$. This can be done using different choices of $\tilde{\psi}_2$ such as a step function arising from a dividing surface, or the normalized signal itself. We will here calculate the systematic error of estimating $\kappa_2$ via an exponential fit to the function:

$$
\tilde{\lambda}_2 = \langle\tilde{\psi}_2(0)\tilde{\psi}_2(\tau)\rangle \ = \ \alpha\mathrm{e}^{-\tau\kappa_2}+\sum_{i>2}a_i^2\mathrm{e}^{-\tau\kappa_i} \tag{62}
$$

using a set of $m$ mutually different lagtimes $\tau_j \in \{\tau_1, ..., \tau_m\}$ in ascending order, $\tau_j < \tau_{j+1}$. For the sake of quantifying the systematic error, we may consider the exponential fit to be implemented via a linear fit to the logarithmized data:

$$
\begin{aligned}
z(\tau) &= \ln\langle\tilde{\psi}_2(0)\tilde{\psi}_2(\tau)\rangle \\
&= \ln[\alpha\mathrm{e}^{-\tau\kappa_2}+\sum_{i>2}a_i^2\mathrm{e}^{-\tau\kappa_i}]
\end{aligned} \tag{63}
$$

A simple linear regression algorithm can then be expressed as:

$$
\begin{aligned}
\tilde{\kappa}_{2,\mathrm{fit}} &= \frac{\mathbb{E}[\tau_j]\mathbb{E}[z(\tau_j)]-\mathbb{E}[\tau_j z(\tau_j)]}{\mathrm{Var}(\tau_j)} \\
&= \frac{\mathbb{E}[(\mathbb{E}[\tau_j]-\tau_j)z(\tau_j)]}{\mathrm{Var}(\tau_j)} \\
&= \frac{\sum_{j=1}^{m}(\bar{\tau}-\tau_j)z(\tau_j)}{m\,\mathrm{Var}(\tau_j)}
\end{aligned} \tag{64}
$$

with expectation of lagtimes

$$
\bar{\tau} = \mathbb{E}[\tau_j] = \frac{1}{m}\sum_{j=1}^{m}\tau_j \tag{65}
$$

and variance of lagtimes

$$\mathrm{Var}(\tau) = \mathbb{E}[(\tau_j - \bar{\tau})^2] = \frac{1}{m}\sum_{j=1}^{m} \tau_j^2 - \bar{\tau}^2. \tag{66}$$

This results in

$$\begin{aligned}
\tilde{\kappa}_{2,\mathrm{fit}} &= \frac{\sum_{j=1}^{m}(\bar{\tau}-\tau_j)\ln[\alpha \mathrm{e}^{-\tau_j\kappa_2} + \sum_{i>2} a_i^2 \mathrm{e}^{-\tau_j\kappa_i}]}{m\,\mathrm{Var}(\tau)} \\
&= \frac{\sum_{j=1}^{m}(\bar{\tau}-\tau_j)\ln[\mathrm{e}^{-\tau_j\kappa_2}\left(\alpha + \sum_{i>2} a_i^2 \mathrm{e}^{-\tau_j(\kappa_i-\kappa_2)}\right)]}{m\,\mathrm{Var}(\tau)} \\
&= \frac{\sum_{j=1}^{m}(\bar{\tau}-\tau_j)\ln \mathrm{e}^{-\tau_j\kappa_2}}{m\,\mathrm{Var}(\tau)} + \frac{\sum_{j=1}^{m}(\bar{\tau}-\tau_j)\ln\left(\alpha + \sum_{i>2} a_i^2 \mathrm{e}^{-\tau_j(\kappa_i-\kappa_2)}\right)}{m\mathrm{Var}(\tau)} \\
&= \kappa_2 \frac{-\frac{1}{m}\sum_{j=1}^{m}(\bar{\tau}-\tau_j)\tau_j}{\mathrm{Var}(\tau)} + \frac{\sum_{j=1}^{m}(\bar{\tau}-\tau_j)\ln\left(\alpha + \sum_{i>2} a_i^2 \mathrm{e}^{-\tau_j(\kappa_i-\kappa_2)}\right)}{m\mathrm{Var}(\tau)} \\
&= \kappa_2 + \frac{\sum_{j=1}^{m}(\bar{\tau}-\tau_j)\ln\left(\alpha + \sum_{i>2} a_i^2 \mathrm{e}^{-\tau_j(\kappa_i-\kappa_2)}\right)}{m\mathrm{Var}(\tau)}
\end{aligned} \tag{67}$$

and the estimation error is given by

$$\Delta\kappa_{2,\mathrm{fit}} = \tilde{\kappa}_{2,\mathrm{fit}} - \kappa_2 = \frac{\sum_{j=1}^{m}(\bar{\tau}-\tau_j)\ln\left(\alpha + \sum_{i>2} a_i^2 \mathrm{e}^{-\tau_j(\kappa_i-\kappa_2)}\right)}{m\mathrm{Var}(\tau)} \tag{68}$$

We simplify further

$$\begin{aligned}
\Delta\kappa_{2,\mathrm{fit}} &= \frac{\sum_{j=1}^{m}(\bar{\tau}-\tau_j)\ln\left(\alpha(1 + \sum_{i>2}(a_i^2/\alpha) \mathrm{e}^{-\tau_j(\kappa_i-\kappa_2)}\right)}{m\mathrm{Var}(\tau)} \\
&= \frac{\sum_{j=1}^{m}(\bar{\tau}-\tau_j)\ln\alpha}{m\mathrm{Var}(\tau)} + \frac{\sum_{j=1}^{m}(\bar{\tau}-\tau_j)\ln\left(1 + \sum_{i>2}(a_i^2/\alpha) \mathrm{e}^{-\tau_j(\kappa_i-\kappa_2)}\right)}{m\mathrm{Var}(\tau)}
\end{aligned}$$

and use that $\sum_{j=1}^{m}(\bar{\tau}-\tau_j) = 0$ so that

$$\Delta\kappa_{2,\mathrm{fit}} = \sum_{j=1}^{m} \frac{(\bar{\tau}-\tau_j)}{m\mathrm{Var}(\tau)} \ln\left(1 + \sum_{i>2}(a_i^2/\alpha)\mathrm{e}^{-\tau_j(\kappa_i-\kappa_2)}\right) \tag{69}$$

remains. This expression can be bounded from above by keeping only all positive summands with times $\tau_1, ..., \tau_l < \bar{\tau}$ where we used the increasing ordering of the times and find that

$$0 < \Delta\kappa_{2,\mathrm{fit}} < \sum_{j=1}^{l} \frac{(\bar{\tau}-\tau_j)}{m\mathrm{Var}(\tau)} \ln\left(1 + \sum_{i>2}(a_i^2/\alpha)\mathrm{e}^{-\tau_j(\kappa_i-\kappa_2)}\right) \tag{70}$$

and then replace all summands by the largest one, which is given by $j = 1$

$$\begin{aligned}
0 < \Delta\kappa_{2,\mathrm{fit}} &< \frac{l}{m}\frac{(\bar{\tau}-\tau_1)}{\mathrm{Var}(\tau)} \ln\left(1 + \sum_{i>2}(a_i^2/\alpha)\mathrm{e}^{-\tau_1(\kappa_i-\kappa_2)}\right) \\
&< \frac{m-1}{m}\frac{(\bar{\tau}-\tau_1)}{\mathrm{Var}(\tau)} \ln\left(1 + \sum_{i>2}(a_i^2/\alpha)\mathrm{e}^{-\tau_1(\kappa_i-\kappa_2)}\right)
\end{aligned} \tag{71}$$

and bound the number of positive summands via $l \leq m-1$. Using that the rates $\kappa_i > \kappa_2$ are ordered we can derive a bound that again only depends on the gap $\kappa_3 - \kappa_2$ and the chosen lag times $\tau_i$

$$0 < \Delta\kappa_{2,\mathrm{fit}} \;<\; \frac{m-1}{m}\frac{(\bar{\tau}-\tau_1)}{\mathrm{Var}(\tau)}\ln\left(1+\mathrm{e}^{-\tau_1(\kappa_3-\kappa_2)}\frac{1-\alpha}{\alpha}\right). \tag{72}$$

Lastly using Samuelson's inequality and $(a+b)^2 \geq 2ab$ we can bound this by

$$0 < \Delta\kappa_{2,\mathrm{fit}} < \frac{(m-1)^2}{m(\tau_m-\bar{\tau})}\ln\left(1+\mathrm{e}^{-\tau_1(\kappa_3-\kappa_2)}\frac{1-\alpha}{\alpha}\right) \tag{73}$$

without knowledge about the variance.

It is important to note that the error is now dominated by an exponential decay in the gap between 2nd and 3rd timescale $\kappa_3 - \kappa_2$ and also decays exponentially in the minimal lagtime $\tau_1$. As expected, the error vanishes for the limit of a perfect reaction coordinate ($\alpha \to 0$).

In order to obtain a more practical expression let us consider that a series of lagtimes is used that obeys the form $(k\tau,\, 2k\tau,\, ...,\, mk\tau)$ for some $k \in \mathbb{R}^+$. In this case, we obtain the explicit bound:

$$\begin{aligned} 0 < \Delta\kappa_{2,\mathrm{fit}} \;&<\; \frac{2(m-1)}{mk\tau}\ln\left(1+\mathrm{e}^{-\tau_1(\kappa_3-\kappa_2)}\frac{1-\alpha}{\alpha}\right) \\ &<\; \frac{2}{k\tau}\frac{1-\alpha}{\alpha}\mathrm{e}^{-\tau_1(\kappa_3-\kappa_2)}. \end{aligned} \tag{74}$$

In the special case of using two lagtimes for the fit with $\tau_1 = \tau$ and $\tau_2 = 2\tau$, we get

$$0 < \Delta\kappa_{2,\mathrm{fit}} \;<\; \frac{1}{\tau}\frac{1-\alpha}{\alpha}\left(\mathrm{e}^{-\tau_1(\kappa_3-\kappa_2)}\right) \tag{75}$$

and even in the worst case of no time scale separation $\kappa_3 = \kappa_2$ we get:

$$0 < \Delta\kappa_{2,\mathrm{fit}} < \frac{1}{\tau}\ln\frac{1}{\alpha}. \tag{76}$$

Finally, the case of a single-$\tau$ estimation can be recovered by the choice of $\tau_1 = 0$ and $\tau_2 = \tau$:

$$0 < \Delta\kappa_{2,\mathrm{fit}} \;<\; \frac{1}{\tau}\ln\frac{1}{\alpha}. \tag{77}$$

Note, that in the absence of statistical uncertainty it is theoretically always better to replace the multi-$\tau$ estimation by a 2-timescale estimation and use the two largest lagtimes $\tau_{m-1}$ and $\tau_m$. In practice this multi-$\tau$ estimators with more than two lagtimes are still recommended in order to diminish the effect of statistical uncertainty.

## IV. OBTAINING MICROSCOPIC TRANSITION RATES $k_{AB}, k_{BA}$ USING PCCA+

In order to convert a relaxation rate $\kappa_2$ to microscopic (state-to-state) transition rates $\kappa_{AB}$ and $\kappa_{BA}$, we need to decompose $\kappa_2$ according to the probability to be in $A$ and $B$, $\pi_A$ and $\pi_B$. For the two-state case this can be achieved based on the estimated eigenfunctions, $\hat{\psi}_1 = \psi_1 = 1$ and $\hat{\psi}_2$, following PCCA+ [3]. We seek state membership functions $\chi_A(y)$ and $\chi_B(y)$ that span the eigenfunctions $\hat{\psi}_1, \hat{\psi}_2$:

$$\begin{aligned} \hat{\psi}_1 &= a_{11}\chi_A(y) + a_{12}\chi_B(y) \\ \hat{\psi}_2 &= a_{21}\chi_A(y) + a_{22}\chi_B(y) \end{aligned} \tag{78}$$

We can write this as a matrix-vector product:

$$\begin{pmatrix} \hat{\psi}_1 \\ \hat{\psi}_2 \end{pmatrix} = \begin{pmatrix} a_{11} & a_{12} \\ a_{21} & a_{22} \end{pmatrix}\begin{pmatrix} \chi_A \\ \chi_B \end{pmatrix} \tag{79}$$

and using the matrix $B = A^{-1}$, rewrite this as:

$$\begin{pmatrix} \chi_A \\ \chi_B \end{pmatrix} = \begin{pmatrix} b_{11} & b_{12} \\ b_{21} & b_{22} \end{pmatrix} \begin{pmatrix} \psi_1 \\ \psi_2 \end{pmatrix} \tag{80}$$

To be able to determine the coefficients we need to evaluate the functions $\chi$ and $\psi$ at two points $y_1$ and $y_2$. This yields four equations which can be written again in matrix form:

$$\begin{pmatrix} \chi_A(y_1) & \chi_A(y_2) \\ \chi_B(y_1) & \chi_B(y_2) \end{pmatrix} = \begin{pmatrix} b_{11} & b_{12} \\ b_{21} & b_{22} \end{pmatrix} \begin{pmatrix} \psi_1(y_1) & \psi_1(y_2) \\ \psi_2(y_1) & \psi_2(y_2) \end{pmatrix} \tag{81}$$

we choose $x_1$ and $x_2$ to be the extreme values of $\psi$ and take them as representatives for the states $A$, $B$. Then:

$$\begin{aligned} \begin{pmatrix} b_{11} & b_{12} \\ b_{21} & b_{22} \end{pmatrix} &= \begin{pmatrix} 1 & 0 \\ 0 & 1 \end{pmatrix} \begin{pmatrix} 1 & 1 \\ \psi_2(y_1) & \psi_2(y_2) \end{pmatrix}^{-1} \\ &= \frac{1}{\psi_2(y_2) - \psi_2(y_1)} \begin{pmatrix} \psi_2(y_2) & -1 \\ -\psi_2(y_1) & 1 \end{pmatrix}. \\ &= \frac{1}{\max \psi_2 - \min \psi_2} \begin{pmatrix} \max \psi_2 & -1 \\ -\min \psi_2 & 1 \end{pmatrix} \end{aligned} \tag{82}$$

and hence:

$$\begin{aligned} \begin{pmatrix} \chi_A \\ \chi_B \end{pmatrix} &= \frac{1}{\max \psi_2 - \min \psi_2} \begin{pmatrix} \max \psi_2 & -1 \\ -\min \psi_2 & 1 \end{pmatrix} \begin{pmatrix} 1 \\ \psi_2 \end{pmatrix} \\ \chi_A(x) &= \frac{\max \psi_2 - \psi_2(y)}{\max \psi_2 - \min \psi_2} \\ \chi_B(x) &= \frac{\psi_2(x) - \min \psi_2}{\max \psi_2 - \min \psi_2}. \end{aligned} \tag{83}$$

We see that $\chi_A(y)$ are fuzzy membership functions:

$$\chi_A(y) + \chi_B(y) = 1 \tag{84}$$

And using

$$A = \begin{pmatrix} 1 & 1 \\ \min \psi_2 & \max \psi_2 \end{pmatrix} \tag{85}$$

we can express $\psi_1$ and $\psi_2$ exactly as linear combinations of these memberships, consequently $\chi_A$ and $\chi_B$ are a decomposition of state space towards the states $A$ and $B$ according to which we can reproduce $\hat{\psi}_2$ optimally, and thus the rate optimally, and with the rate estimation procedure given above even asymptotically exactly. Therefore, $\chi_A$ and $\chi_B$ are optimal choices as memberships for $A$ and $B$.

### Effect of filtering on rate estimates

In order to test the effect of time-binning on the quality of a rate estimate, we have constructed a diffusion process in a one-dimensional two-well potential with a dominant relaxation rate $\kappa_2 = 0.349$ (timescale $t_2 = \kappa_2^{-1} = 286.5$ time steps) and fast relaxation rates of $\kappa_3 = 0.115$ (timescale $t_3 = \kappa_3^{-1} = 8.6$ time steps) or faster. A long simulation trajectory ($10^6$ time steps) was generated and time-binned using window lengths of 10, 100 and 1000 time steps. Fig. 1 left shows the normalized autocorrelation function of the resulting signal, $\tilde{\lambda}_2(\tau) = \langle y_t y_{t+\tau} \rangle$. It is seen that for the original signal, $\tilde{\lambda}_2(\tau)$ shows

an initial fast decay due to the fast processes and then decays single exponentially with rate $\kappa_2$. Time-binned signals show a longer non-exponential phase in the beginning that also leads over to a single-exponential decay with rate $\kappa_2$. The non-exponential phase lasts a short multiple of the binning time. For example, for the binning time 100 time steps, the single-exponential phase is found at lagtimes of about $\tau = 150$ time steps or greater. For the binning time 1000 steps, lagtimes of $\tau = 1500$ or greater are needed, which is unfortunately much larger than the timescale of the process itself. Fig. 1 right shows the effect of this modification of $\tilde{\lambda}_2(\tau)$ on the MSM rate estimate $\tilde{\kappa}_2 = -\tau^{-1} \ln \tilde{\lambda}_2(\tau)$. It is seen that a binning time of 10 time step yields a small error of the estimated rate, while a binning time of 100 or more time steps already yields a large error. We recommend that the binning time used is a factor of 10 smaller than the timescale of interest, indicated by the long-$\tau$ estimate of $\tilde{t}_2(\tau) = \tilde{\kappa}_2^{-1}(\tau)$.

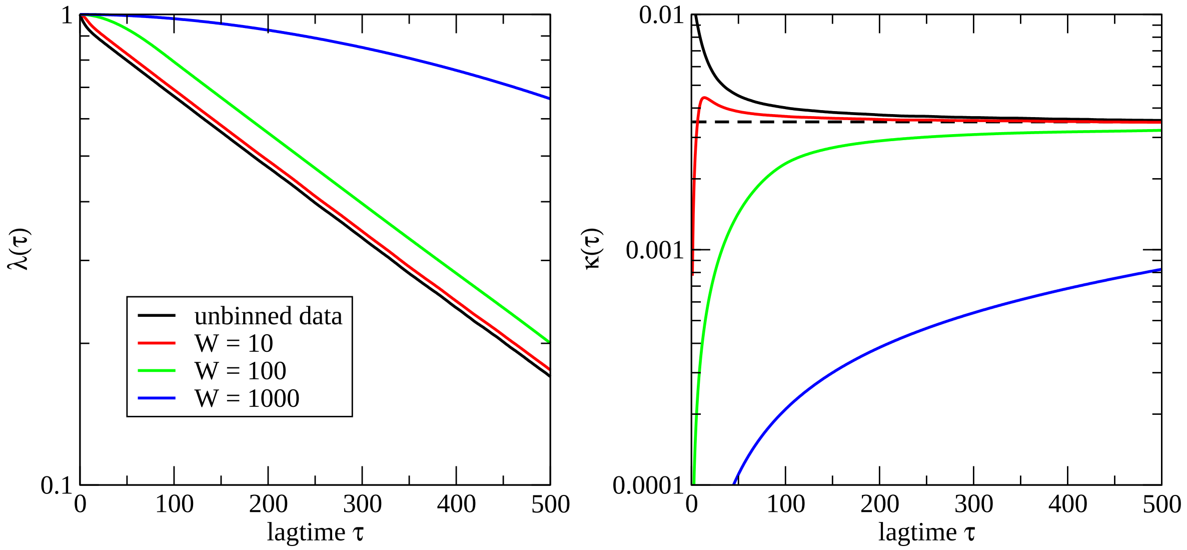


Figure 1: Test of the effect of time binning on the filtering theory on a diffusion process in a two-well potential. Left: $\tilde{\lambda}_2(\tau) = \langle y_t y_{t+\tau} \rangle$ for different window sizes. Right: apparent rates $\tilde{\kappa}_2(\tau) = -\tau^{-1} \ln \tilde{\lambda}_2(\tau)$. The exact rate is shown as a dashed black line.

**Comparison of rates using different dividing surfaces and spectral estimator**

Fig. 2 shows a comparison of the estimated rates from the dividing surface estimator with different choices of the dividing surface and the spectral estimator, for the apo-myoglobin data reported in the main manuscript. All estimates are made at a lagtime $\tau = 15\,ms$. The direct 50 kHz dataset is shown in the left panel, while the filtered dataset that has been binned to 1 kHz is shown in the right panel. Row (a) reports again the histograms and partial probability densities of the two slowest-interconverting states that are also given in the main manuscript. Row (b) reports the estimate of the relaxation rate $\kappa_2$ for different choices of the dividing surface. This result shows that, as expected from the theory, the dividing surface estimate and the spectral estimate agree as long as reasonable choices for the dividing surface are made. When the dividing surface is chosen too far to the "left" or "right", the content of state $B$ and $A$, respectively, is so small that numerical errors are introduced and the dividing surface rate estimate becomes unreliable. Row (c) reports the estimates of the microscopic transition rates $k_{AB}$ and $k_{BA}$ for different choices of the dividing surface. It is seen that the estimate of spectral estimator and dividing surface estimator meet at one point. Since the dividing surface rate constants are produced by splitting the rate $\kappa_2 = k_{AB} + k_{BA}$ in a way that depends on how much aggregate probability of $\mu^o(o)$ is "left" and and "right" of the dividing surface, and since the estimate of $\kappa_2$ is unbiased, there always exists one choice of the dividing surface that yields the correct microscopic rates $k_{AB}$ and $k_{BA}$. However, this is an error compensation effect based on the fact that for this the amount of probability from the "right" state overlapping to the "left" side of the dividing surface (and vice versa) happen to neutralize each other in the estimate of $k_{AB}$ and $k_{BA}$. There is no indicator in the data what this choice is because generally $k_{AB}$ and $k_{BA}$ will not be equal as in the present case. On the other hand, the spectral estimate of the microscopic transition rates is unbiased and does not need a definition of dividing surface.

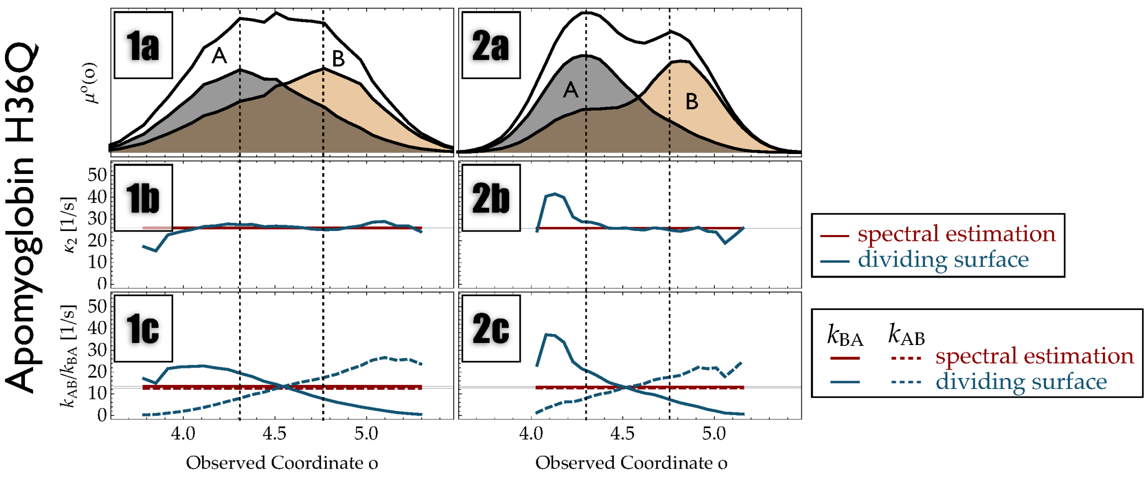


Figure 2: Comparison of the estimated rates from the dividing surface estimator with different choices of the dividing surface and the spectral estimator, for the apo-myoglobin data reported in the main manuscript. All estimates are made at a lagtime $\tau = 15\,ms$ (1) Direct 50 kHz dataset. (2) Filtered dataset that has been binned to 1 kHz. (a) Histograms and partial probability densities of the two slowest-interconverting states. (b) Estimate of the relaxation rate $\kappa_2$ for different choices of the dividing surface. (c) Estimate of the microscopic transition rates $k_{AB}$ (dashed) and $k_{BA}$ (solid) for different choices of the dividing surface.

**Robust eigenvector estimation**

Although statistical issues were largely not considered in this manuscript, there is one point in the estimation procedure where statistical uncertainty can become crucial: In Eq. (83), the partital probability distributions of substates $A$ and $B$ are estimated from the dominant eigenvector $\hat{\boldsymbol{\psi}}_2$, and in particular involve its minimum and maximum values $\min \psi_2$ and $\max \psi_2$. These minimum and maximum values typically lie where the observed signal has its minimum and maximum value, and therefore in regions with poor statistics.

In order to obtain a reliable estimate of the partial probability distributions $\mu_A(o)$ and $\mu_B(o)$ and therefore also of the microscopic rate constants $k_{AB}$ and $k_{BA}$, one needs to ensure that the statistical uncertainty of the values $\min \psi_2$ and $\max \psi_2$ is not too large. This can be ensured by designing the binning of the observed coodinate $o$ such that the first and last bin each contain at least a fraction $p_{min}$ of the data points. Here, we choose $p_{min} = 0.0005$ (0.05% in each state, equivalent to 0.1% in both state).

To see that this choice is not arbitrary, and that the results are robust with respect to changes of this choice, consider Fig. 3. Fig. 3 shows the results of the decomposition in the case of the apo-myoglobin (see Fig. 5 in the main text) with filtering $W = 1$ ms. We plot the results for $\pi_A$, the membership of state $A$, $\chi_A(o)$, and the partial probabilities $\mu_A(o)$ and $\mu_B(o)$ depending on the choice of the fraction $p_{min}$. For $p_{min} > 10^{-5}$ the fluctuations for the total stationary probability of state $A$ are within a 1% range (s. Fig. 3 a) and so the estimates of the microscopic rates $\kappa_{AB}$ and $\kappa_{BA}$ stabilize. If we increase the cutoff further, also the noise in the estimated memberships reduces and we get a more stable estimate of the shape of the single states $A$ and $B$ (s. Fig. 3 b). In particular, Fig. 3d shows that for too small a fraction $p_{min} \approx 10^{-6}$, statistical effects lead to an apparent bimodel shape in the distribution of the $B$ state, which disappears when more data is included in the first and last discretization bin.

For the main text we settled on a cutoff of 0.1% (0.05% on each side) that seemed a reasonable compromise to stabilize the estimation while not removing too much data.

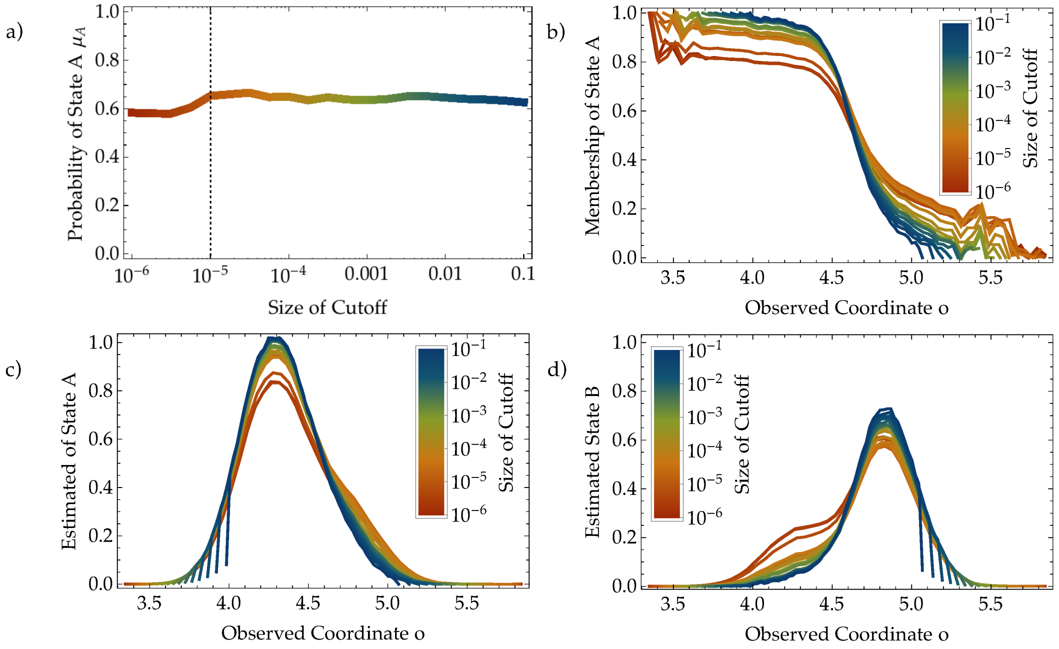


Figure 3: Sensitivity of state decomposition on extended binning. Estimation result for the apo-myoglobin with filtering (s. Fig. 3 and Fig. 5 in the main text) depending on the total cutoff choice for the left and right most bins combined. (a) Total stationary probability $\pi_A$ of being in state $A$ (left). After about $10^{-5}$ the fluctuation are below 1%. (b) Estimated membership of state $A$ depending on the cutoff. With increasing cutoff the fluctuations at the left and right most states decrease and suggest a more stable decomposition. (c) + (d) Estimated shape of state $A$ and $B$ depending on the cutoff. With increasing cutoff an apparent bimodel shape disappears toward an unsymmetric but unimodal shape. Very large cutoffs start to affect the overall shape of the distribution.

---


[1] David Chandler. Statistical mechanics of isomerization dynamics in liquids and the transition state approximation. *The Journal of Chemical Physics*, 68(6):2959–2970, 1978.

[2] John D. Chodera, Phillip J. Elms, William C. Swope, Jan-Hendrik Prinz, Susan Marqusee, Carlos Bustamante, Frank Noé, and Vijay S. Pande. A robust approach to estimating rates from time-correlation functions. *http://arxiv.org/abs/1108.2304*, 2011.

[3] P. Deuflhard and M. Weber. Robust Perron cluster analysis in conformation dynamics. *ZIB Report*, 03-09, 2003.

[4] John A. Montgomery, David Chandler, and Bruce J. Berne. Trajectory analysis of a kinetic theory for isomerization dynamics in condensed phases. *The Journal of Chemical Physics*, 70(9):4056–4066, 1979.

[5] L. Onsager. Reciprocal relations in irreversible processes II. *Phys. Rev.*, 38:2265–2279, 1931.
